# Supplementary material for: A 1D-0D-3D coupled model for simulating blood flow and transport processes in breast tissue
Source: arXiv:2201.05392 source file (2022-01-14)
Supplement: Supplementary file 1 [file multiscale_appendix.tex]

%\newpage
\appendix 

\section{Data set description} \label{Appendix:Data}
The estimated parameter values for the vessels in the simulations are reported here in Table~\ref{tab:dataVascTree}.
{\small
\begin{table}[!h]
\caption{\label{tab:dataVascTree} 
    Data for the thoracic arteries as well as the breast network. 
    The radii $r$ of the thoracic arteries can be found in \cite{?}. 
    The elasticity parameters are estimated. 
    In the case of the breast network, only the wall thickness $h$ and the elasticity $E$ are relevant, since the lengths and radii are given by the data set from \cite{wu2020patient}. 
    For simplicity, we use for each vessel in the breast network the same wall thickness and the elasticity parameter.
    }
	\begin{tabular}{|l|c|c|c|c|c|}
	%	\hline
		\hline
		\textbf{Vessel name} & \textbf{Id} &  $l\,\left[\unit{cm} \right]$ &  $r\, \left[ \unit{cm} \right]$ & $h\, \left[ \unit{cm} \right]$ & $E\, \left[ \unit{MPa} \right]$\\
		\hline
		\hline
		Subclavian artery (I) & $7$ & $1.70$ & $0.423$ & $0.067$ & $0.4$ \\
		\hline
		Subclavian artery (II) & $34$ & $1.70$ &  $0.423$ & $0.067$ &  $0.4$\\
		\hline
		Brachial artery (I) & $15$ & $40.5$ & $0.403$ & $0.067$ & $0.4$ \\
		\hline
		Brachial artery (II) & $35$ & $1.70$ & $0.403$ & $0.067$ & $0.4$ \\
		\hline
		Internal thoracic artery (I) & $36$ & $2.5$ & $0.06$ & $0.005$ & $1.3$ \\
		\hline
		Internal thoracic artery (II) & $37$ & $2.5$ & $0.06$ & $0.005$ & $1.3$ \\
		\hline
		Internal thoracic artery (III) & $38$ & $2.0$ & $0.06$ & $0.005$ & $1.3$ \\
		\hline
		Internal thoracic artery (IV) & $39$ & $0.5$  & $0.06$ & $0.005$ & $1.3$ \\
		\hline
		Internal thoracic artery (V) & $40$ & $0.5$ & $0.06$ & $0.005$ & $1.3$ \\
		\hline
		Internal thoracic artery (VI) & $41$ & $5.0$ & $0.06$ & $0.005$ & $1.3$ \\
		\hline
		Lateral thoracic artery (I) & $42$ & $2.5$ & $0.06$ & $0.005$ & $1.3$ \\
		\hline
		Lateral thoracic artery (II) & $43$ & $2.5$ & $0.06$ & $0.005$ & $1.3$ \\
		\hline
		Lateral thoracic artery (III) & $44$ & $2.5$ & $0.06$ & $0.005$ & $1.3$ \\
		\hline
		Lateral thoracic artery (IV) & $45$ & $7.0$ & $0.06$ & $0.005$ & $1.3$ \\
		\hline
		Breast network & --- & ----- & $0.013-0.042$ & $0.005$ & $1.3$  \\
		\hline
	%	\hline
	\end{tabular}
\end{table}
}

\section{Viscosity}
\label{sec:appendix:viscosity}

Red blood cells govern the viscosity of blood, significantly. 
As the red blood cells have to deform such that they can move through capillaries, the viscosity varies within the microvascular network.
A quantitative relationship between the vessel diameter $D$ is given by the following formula for the in vivo viscosity
$\mu_{\mathrm{bl}}\;\left[ \unit{Pa \cdot s} \right]$, see \cite{pries1996biophysical}:
\begin{equation}
\label{eq:viscosity}
\mu_{\mathrm{bl}}\left( D \right) = \mu_{\mathrm{p}} \left( 1+ \left( \mu_{0.45} -1 \right)
\frac{\left(1-H \right)^C-1}{\left(1-0.45 \right)^C-1} \cdot \left( \frac{D}{D-1.1} \right)^2 \right)
\cdot \left( \frac{D}{D-1.1} \right)^2.
\end{equation}
In \eqref{eq:viscosity}, the diameter $D$ is dimensionless. The physical diameter $d\;\left[\unit{\mu m}\right]$
has to be divided by $1.0\;\unit{\mu m}$ to obtain $D$. Here, $\mu_{\mathrm{p}}\;\left[ \unit{Pa \cdot s} \right]$ denotes the viscosity of blood plasma, and $H$ stands for the discharge hematocrit, which is defined by the ratio between the volume of the red blood cells and the total blood volume. The apparent viscosity $\mu_{0.45}$ is given by:
\[
\mu_{0.45} = 6.0 \exp\left(-0.085 \cdot D \right) + 3.2 - 2.44 \exp\left(-0.06 \cdot D^{0.645} \right),
\]
and $C$ is a coefficient determining the influence of $H$ on $\mu_{\mathrm{bl}}$:
\[	
C = \left( 0.8 + \exp\left(-0.075 \cdot D \right) \right) \left(-1 + \frac{1}{1 + 10^{-11} D^{12}} \right)
+ \frac{1}{1 + 10^{-11} D^{12}}.
\]
In this context, one should be aware of the fact that the constitutive relationship \eqref{eq:viscosity} is known to hold for human blood.

\section{Reduced 1D and 0D models} \label{Appendix:Model}
The multiscale model developed here uses various well established submodules, which are summarized here for convenience.
The reduced 1-dimensional nonlinear model and its linearized variant are given in sections~\ref{sec:appendix:nonlinearmodel} and \ref{sec:appendix:linearizedmodel}, followed by the lumped 0D Windkessel model in Section~\ref{sec:appendix:windkessel-model}.

\subsection{Nonlinear 1D model}\label{sec:appendix:nonlinearmodel}
First, the most accurate 1D model, which consists of a set of nonlinear equations, is considered.
Consider a single vessel $\Omega_i,\;i \in I_{non}$ with a length of $l_i$. We use a one-dimensional model to describe the propagation of pressure waves and solutes. For each curve parameter $z \in \left[0,l_i\right]$ and a time point $t>0$, we consider the section area $A_i\left(z,t\right)\;\left[ \unit{cm}^2 \right]$, flow rate $Q_i\left(z,t\right)\;\left[ \unitfrac{cm^3}{s} \right]$ and averaged concentration $\Gamma_i\left(z,t\right)\;\left[ \unitfrac{mmol}{cm} \right]$. Averaging the Navier--Stokes equations and a convection diffusion equation across the section area and using \eqref{Ass:BloodTurbulent}, one obtains a first order PDE-system governing $A_i,\;Q_i$ and $\Gamma_i$, see \cite{vcanic2003mathematical,hughes1973one,d2007multiscale}:
\begin{align}
    \label{eq:masscon}
    \frac{\partial A_i}{\partial t} + \frac{\partial Q_i}{\partial z} = 0, & \; z \in \left(0,l_i \right),\;t>0, \\
    \label{eq:momentumcon}
    \frac{\partial Q_i}{\partial t} + \frac{\partial}{\partial z}\left( \frac{Q_i^2}{A_i} \right) + \frac{A_i}{\rho}\frac{\partial P_i}{\partial z} + 2 \cdot \left( \gamma+2 \right) \cdot \frac{\mu\left( 2 \cdot R_i \right)}{\rho} \cdot \frac{Q_i}{A_i} =0,
                                                                           & \; z \in \left(0,l_i \right),\;t>0, \\
    \label{eq:transport}
    \frac{\partial \Gamma_i}{\partial t} + \frac{\partial}{\partial z}\left( \frac{Q_i}{A_i}\Gamma_i \right) = 0,
                                                                           & \; z \in \left(0,l_i \right),\;t>0.
\end{align}
Here, $\rho\;\left[\unitfrac{g}{cm^3} \right]$ is the density of blood. Since blood is assumed to be incompressible, $\rho$ is taken to be constant. The viscosity of blood $\mu$ is given by \eqref{eq:viscosity}, $R_i\;\left[ \unit{cm} \right]$ is the radius of the vessel $\Omega_i$. The choice of the dimensionless parameter $\gamma$ depends on the type of flow and the radial velocity profile. According to \cite{vcanic2003mathematical} and \cite[Chapter 2 and Section 6.1]{d2007multiscale} $\gamma = 9$ is an appropriate choice for a turbulent flow \cite{smith2002anatomically}. $P_i\;\left[ \unit{Ba} \right]$ denotes the fluid pressure on the vessel surface. To complete the system, we present a simple FSI-model that relates the section area $A_i$ and the pressure $P_i$. The FSI model can be derived from the Young Laplace
equation \cite{olufsen1999structured,toro2016brain}:
\begin{equation}
    \label{eq:PressureAreaRelation}
    P_i(z,t) = G_{0,i} \left( \sqrt{\frac{A_{i}}{A_{0,i}}} - 1 \right),\qquad G_{0,i} = \frac{\sqrt{\pi} \cdot h_{0,i} \cdot
        E_i}{\left(1-\nu^2\right) \cdot \sqrt{A_{0,i}}},
\end{equation}
where $E_i$ is the Young modulus, $A_{0,i}$ stands for the section area at rest, $h_{0,i}$ is the vessel thickness and $\nu$ is the Poisson ratio. Due to the fact that biological tissue is practically incompressible, $\nu$ is
chosen as $\nu = 0.5$ \cite[Chapter 10]{Quarteroni}. Equation \eqref{eq:PressureAreaRelation} is based on the assumption that the vessel wall is instantaneously in equilibrium with the forces acting on it.

Analyzing the characteristics of this system of equations \eqref{eq:masscon}-\eqref{eq:transport}, it can be shown that changes in pressure, flow rate, and the concentration variable are propagated by $W_{1,i}$, $W_{2,i}$ and $W_{3,i}$:
\begin{align}
    \label{eq:W1}
    W_{1,i} & = -\frac{Q_i}{A_i} + 4 \sqrt{ \frac{G_{0,i}}{2 \rho} } \left( \left( \frac{A_i}{ A_{0,i} } \right)^{\frac 14} - 1 \right) = -v_i + 4 \cdot \left( c \left(A_i \right)
    -c\left(A_{0,i} \right) \right),                                                                                                                                                \\
    \label{eq:W2}
    W_{2,i} & = \frac{Q_i}{A_i}  + 4 \sqrt{ \frac{G_{0,i}}{2 \rho} } \left( \left( \frac{A_i}{ A_{0,i} } \right)^{\frac 14} - 1 \right) = v_i + 4 \cdot \left( c \left(A_i \right)
    -c\left(A_{0,i} \right) \right),                                                                                                                                                \\
    \label{eq:W3}
    W_{3,i} & = \frac{\Gamma_i}{A_i}.
\end{align}
$v_i\;\left[ \unitfrac{cm}{s} \right]$ is the flow velocity in $\Omega_i$ and $c \left(A_i \right)\;\left[ \unitfrac{cm}{s} \right]$ is the characteristic wave speed in $\Omega_i$. According to \cite{Riviere} it can be shown that assuming $v_i \ll c \left(A_i \right)$, the PDE-system \eqref{eq:masscon}-\eqref{eq:momentumcon} is strictly hyperbolic. Furthermore, it is revealed that $W_{1,i}$ can be compared to a wave moving in a negative direction and that $W_{2,i}$ is a wave moving in a positive direction. The flow direction of $W_{3,i}$ depends on the sign of the velocity field $v_i$. This information is crucial to couple the single vessels and impose boundary conditions in a consistent manner.

A branching point is referred to as $n$-furcation, if $n$ vessels are coupled at this branching point.
In order to couple $n$ vessels at a branching point, we require $3n$ equations to determine the boundary conditions for the adjacent vessels.
For deriving these equations, we follow the considerations, presented in \cite{formaggia2001coupling,koppl2013reduced,masri2021discontinuous}.
Therefore, an index set of the vessels connected at branching point is introduced:
\[
    I_B = \left\{ j_1,\ldots, j_n \right\} \subset I_{non}.
\]
The curve parameters of the corresponding inlets and outlets are denoted by $z_{i_j} \in \left\{0,l_{i_j}\right\}$. One coupling condition is motivated by enforcing mass conservation at the branching point. To achieve this, we demand that the flow rates times the ''outer normal'' $\sigma$ sum up to zero:
\begin{equation}
    \label{eq:masscon_bif}
    \sum_{k \in I_B} \sigma\left( z_k \right) Q_k\left( z_k,t \right) = 0, \;
    \sigma\left( z_k \right) =
    \begin{cases}
        1,\text{ if } z_k = l_k, \\
        -1,\text{ if } z_k = 0.
    \end{cases}
\end{equation}
Further coupling conditions are based on the continuity of the total pressure:
\begin{equation}
    \label{eq:pcon_bif}
    p_{t,j_1}\left( z_{j_1},t \right) = p_{t,k}\left( z_k,t \right),\;
    p_{t,k} = \frac{1}{2} \cdot \rho \cdot \left( \frac{Q_k\left( z_k,t \right)}{A_k\left( z_k,t \right)} \right)^2 + p_k \left( z_k,t \right),\; k \in I_B \setminus \left\{ j_1 \right\}.
\end{equation}
In \cite{formaggia2001coupling} it is shown that the total energy of the system is bounded by boundary conditions and initial conditions, if the continuity of the total pressure is enforced. From \eqref{eq:masscon_bif} and \eqref{eq:pcon_bif}, we obtain $n$ coupling conditions. Thus, $n$ further coupling conditions are required to determine the fluid variables $A_k\left( z_k,t \right)$ and $Q_k\left( z_k,t \right)$. As we know from our characteristic analysis, either $W_{1,k}\left( z_k,t \right)$ or $W_{2,k}\left( z_k,t \right)$ is moving towards the branching point. With $n$ characteristic variables moving towards the $n$-furcation, $n$ additional coupling conditions can be established. This results in a non-linear system of equations that has to be solved for time points of interest. A more detailed description of the system of equations can be found in \cite{formaggia2003one,puelz2017comparison}.

For modeling transport processes through a branching point, we require some further notation. The index set $I_B$ is divided into two disjunctive sets $I_{B_{in}}$ and $I_{B_{out}}$. For these index sets it holds:
\[
    k \in I_{B_{in}} \Longleftrightarrow \left( z_k = 0 \wedge Q_k\left( z_k,t \right) \leq 0 \right) \vee
    \left( z_k = l_k \wedge Q_k\left( z_k,t \right) \geq 0 \right),
\]
and
\[
    k \in I_{B_{out}} \Longleftrightarrow \left( z_k = 0 \wedge Q_k\left( z_k,t \right) > 0 \right) \vee
    \left( z_k = l_k \wedge Q_k\left( z_k,t \right) < 0 \right).
\]
Accordingly, the conservation of solute mass at a branching point can be formulated as follows:
\begin{equation}
    \label{eq:gamma_con_bif}
    N_{in} \left(t\right) = \sum_{k \in I_{B_{in}}} \left| Q_k\left( z_k,t \right) \right| \frac{\Gamma_k\left( z_k,t \right)}{A_k\left( z_k,t \right)} = \sum_{k \in I_{B_{out}}} \left| Q_k\left( z_k,t \right) \right| \frac{\Gamma_k\left( z_k,t \right)}{A_k\left( z_k,t \right)}.
\end{equation}
$N_{in}\;\left[\unitfrac{mmol}{s}\right]$ is the number of particles flowing through the bifurcation within a second. Next, we note that the concentration variables $\Gamma_k\left( z_k,t \right),\;k \in I_{B_{in}}$ can be determined by means of an upwinding method, since the corresponding characteristic variables $W_3\left( z_k,t\right)$ are leaving the inflow vessels and entering the bifurcation. This means that $N_{in}$ can be computed for each time point $t>0$. It remains to determine $\Gamma_k\left( z_k,t \right),\;k \in I_{B_{out}}$. For this purpose, we assume that an instantaneous mixing at the branching point takes place. This means that:
\[
    \frac{\Gamma_k\left( z_k,t \right)}{A_k\left( z_k,t \right)} = W_{3,k}\left( z_k,t \right) \equiv constant, \quad
    \forall k \in I_{B_{out}}.
\]
Taking this into account and using the mass conservation for the fluid system, it holds for $l \in I_{B_{out}}$:
\begin{equation}
    \label{eq:gamma_out}
    \Gamma_l\left( z_l,t \right) = \frac{A_l\left( z_l,t \right)}{\left| Q_l\left( z_k,t \right) \right|} \cdot N_{in} \left(t\right) \cdot \frac{\left| Q_l\left( z_k,t \right) \right)}{\sum_{k \in I_{B_{in}}} \left| Q_k\left( z_k,t \right) \right|} = \frac{A_l\left( z_l,t \right) \cdot N_{in} \left(t\right)}{\sum_{k \in I_{B_{in}}} \left| Q_k\left( z_k,t \right) \right|}.
\end{equation}
This completes the coupling conditions of the nonlinear scheme.

\subsection{Linearized 1D model}\label{sec:appendix:linearizedmodel}

After introducing the nonlinear model, we move one step further down the vascular tree and consider smaller vessels for which a linearized equation is sufficient.
To a vessel $\Omega_i,\;i \in I_{lin}$ of length $l_i$, we assign a pressure variable $p_i\;\left[ Ba \right]$, a flow rate $q_i\;\left[ \unitfrac{cm^3}{s} \right]$ and the averaged concentration variable $\Gamma_i\;\left[ \unitfrac{mmol}{cm} \right]$.
Based on assumption \eqref{Ass:BloodLaminar}, 1D linearized version of \eqref{eq:masscon}-\eqref{eq:transport} is used to model flow and transport within the breast network. 
Its derivation is based on the assumption $A_i \approx A_{i,0}$ and can be found in \cite[Section 6.2.1]{d2007multiscale}:

\begin{align}\label{eq:masscon_lin}
    \frac{\partial p_i}{\partial t} + \frac{1}{\tilde{C}_i}\frac{\partial q_i}{\partial z} = 0, &\quad \; z \in \left(0,l_i \right),\;t>0, \\
    \label{eq:momentumcon_lin}
    \frac{\partial q_i}{\partial t} + \frac{1}{L_i}\frac{\partial p_i}{\partial z} + K_{r,i}  \cdot \frac{q_i}{A_{0,i}}=0,
                                                                                                &\quad \; z \in \left(0,l_i \right),\;t>0, \\
    \label{eq:transport_lin}
    \frac{\partial \Gamma_i}{\partial t} + \frac{\partial}{\partial z}\left( \frac{q_i}{A_{0,i}}\Gamma_i \right) = 0,
                                                                                                &\quad \; z \in \left(0,l_i \right),\;t>0.
\end{align}
The parameters $\tilde{C}_i$, $L_i$ and $k_{r,i}$ represent the wall compliance, inertia and resistance parameter of vessel $\Omega_i$, they are given by:
\[
    \tilde{C}_i = \frac{A_{0,i}}{\rho \cdot c\left( A_{0,i} \right)},\qquad L_i = \frac{\rho}{A_{0,i}}, \qquad  K_{r,i} = 2 \cdot \left( \gamma+2 \right) \cdot \frac{\mu\left( 2 \cdot R_{0,i} \right)}{\rho}.
\]
Here, $R_{0,i}\;\left[\unit{cm} \right]$ is the radius of vessel $\Omega_i$. It is given by $R_{0,i} = \sqrt{A_{0,i}/\pi}$.
Since we assumed laminar and Poiseuille type flow, the parameter $\gamma$ is set to $2$ according to \cite[Section 6.1]{d2007multiscale}.
Again the viscosity parameter $\mu$ is given by \eqref{eq:viscosity} to account for non-Newtonian effects.

Similar to \eqref{eq:masscon}-\eqref{eq:transport} one can show that the first order PDE-system \eqref{eq:masscon_lin}-\eqref{eq:transport_lin} is hyperbolic and that the solution variables can be transformed into characteristic variables $w_{1,i}$, $w_{2,i}$ and $w_{3,i}$. The first two characteristic variables are connected to the fluid variables $p_i$ and $q_i$, and $w_{3,i}$ is related to $\Gamma_i$:
\begin{align}
    \label{eq:w123}
    w_{1,i} & = \frac 12 \left( -\sqrt{ \frac{\tilde{C}_i}{L_i} } p_i + q_i \right),\; w_{2,i} = \frac 12 \left( \sqrt{ \frac{\tilde{C}_i}{L_i} } p_i + q_i \right) \text{ and } w_{3,i} = \frac{\Gamma_i}{A_{0,i}}.
\end{align}
Thereby, $w_{1,i}$ can be compared to a wave moving into negative direction, while $w_{2,i}$ is moving in the opposite direction. The direction of motion of $w_{3,i}$ depends on the sign of $q_i$. As for the non-linear PDE-system \eqref{eq:masscon}-\eqref{eq:transport} this knowledge is important to impose boundary conditions in a meaningful manner.

Coupling $n$ linear flow and transport models \eqref{eq:masscon_lin}-\eqref{eq:transport_lin} at a branching point can be done in a similar way as in the non-linear case. Replacing in \eqref{eq:masscon_bif} $Q_k$ by $q_k$, we obtain the mass conservation equation. The continuity of the total pressure is replaced by the continuity of the fluid pressure \cite{d2007multiscale}:
\[
    p_{j_1}\left( z_{j_1},t \right) = p_{k}\left( z_k,t \right),\quad k \in I_B \setminus \left\{ j_1 \right\}.
\]
Closing the system, the outgoing characteristic variables are extrapolated using \eqref{eq:w123}. This yields a linear system of equations governing the fluid variables at a branching point. The concentration variables are determined similar to \eqref{eq:gamma_con_bif}. Replacing $Q_k$ by $q_k$ and $A_l$ by $A_{0,l}$ in \eqref{eq:gamma_con_bif} the concentration values for the vessels in $I_{B_{out}}$ are obtained. The concentration values for the vessels in $I_{B_{in}}$ are obtained by extrapolating the outgoing characteristics.

\subsection{0D Windkessel model}
\label{sec:appendix:windkessel-model}
We consider a vessel $\Omega_i$ with $i \in I_{wk}$ and assume that their parametrization is oriented such that $z_i=l_i$ is adjacent to the outlets.
At the outlet of a larger artery $\Omega_i$, the reflections of the pulse waves at the omitted vessels have to be incorporated to be able to simulate realistic pressure and velocity curves.
For this purpose, we assign to each terminal vessel a reflection
parameter $R_{p,i} = R_{1,i} + R_{2,i}$, where $R_{1,i}$ is the resistance parameter of $\Omega_i$ \cite{alastruey2008lumped}:
\[
    R_{1,i} = \frac{\rho \cdot c\left(A_{0,i} \right)}{A_{0,i}}.
\]
This choice depends on artificial reflection at the interface between the 1D and the 0D model is kept to a minimum. $R_{2,i}$ is the resistance parameter for all the vessels that are connected to $\Omega_i$ but not contained in the macrocirculation. The third parameter $C_i$ represents the compliance of the omitted
vessels and is a measure of the ability of these vessels to store a certain blood volume. The triple
$\left(R_{1,i},C_i,R_{2,i} \right)$ is referred to as a ``three-element Windkessel'' model in 
\cite{alastruey2008lumped,Quarteroni}. The values for the Windkessel parameters used in our simulations are listed in \cite[Table 1]{alastruey2007modelling}. In order to describe the dynamics of a Windkessel model, the following ODE has been derived using averaging techniques and an analogy from electrical science \cite{alastruey2007modelling,alastruey2008lumped,marchandise2009numerical}:
\begin{equation} \begin{aligned}
    \label{eq:Outflow}
    C_i \frac{\d p_{c,i}}{\d t} &= \frac{P_i\left(l_i,t\right)-p_{c,i}}{R_{1,i}}-\frac{p_{c,i}-p_v}{R_{2,i}}, \\
    Q_i\left(l_i,t\right) &= \frac{P_i\left(l_i,t\right)-p_{c,i}}{R_{1,i}},\qquad Q_{ven,i} = \frac{p_{c,i}-p_v}{R_{2,i}}. \end{aligned}
\end{equation}
$P_i\left(l_i,t\right) = p_i\left(A_i\left(l_i,t\right)\right)$ is given by \eqref{eq:PressureAreaRelation}. Here, $p_{c,i}$ and $p_v$ are averaged arterial and venous pressures and $Q_{ven,i}$ represents the flow rate from the arterial system into the venous system. Solving \eqref{eq:Outflow} and using the outgoing characteristic variable $W_{2,i}\left(l_i,t\right)$, the boundary conditions for $A_i\left(l_i,t\right)$ and $Q_i\left(l_i,t\right)$ can be determined. Further details can be found, e.g., in \cite{alastruey2007modelling,alastruey2008lumped,marchandise2009numerical}. It remains to model the behavior of the concentration variable at an outlet.

For $\Gamma_i\left( l_i,t \right)$, a concentration variable $c_i\;\left[ \unitfrac{mmol}{cm^3} \right]$ is introduced for the omitted arterial system and to establish a mass balance equation for the solute particles leaving or entering the omitted arterial system:
\[
    \frac{\d}{\d t}\left( V_i\left( t \right) c_i\left( t \right) \right) = N_i\left(t \right) - N_{ven}\left( t\right),
\]
where $N_i\;\left[ \unitfrac{mmol}{s} \right]$ represents the number of particles leaving or entering the terminal 1D vessel per second, while $N_{ven}\;\left[ \unitfrac{mmol}{s} \right]$ denotes the number of particles migrating into the venous system during a second. Moreover, $V_i\;\left[ \unit{cm}^3 \right]$ is the fluid volume contained in the omitted arterial system. It can be computed by means of the following ODE:
\begin{equation}
    \label{eq:V_i}
    \frac{\d V_i}{\d t}  = Q_i\left(l_i,t\right) - Q_{ven,i}\left( t \right).
\end{equation}
To determine $N_i$, we have to check the sign of $Q_i\left(l_i,t\right)$:
\[
    N_i\left( t \right) =
    \begin{cases}
        \frac{\Gamma_i\left( l_i,t \right) Q_i\left( l_i,t \right)}{A_i\left( l_i,t \right)}, &\text{ if } Q_i\left( l_i,t \right) \geq 0, \\
        Q_i\left( l_i,t \right) \cdot c_i\left(t\right), &\text{ if } Q_i\left( l_i,t \right) < 0.
    \end{cases}
\]
Assuming that $Q_{ven,i} \geq 0$, $N_{ven}\left( t\right)$ is given by:
\[
    N_{ven}\left( t\right) = c_i\left( t\right) \cdot Q_{ven,i}\left( t \right) = c_i\left( t\right) \cdot \frac{p_{c,i}-p_v}{R_{2,i}}.
\]
Summarizing the above equations, the following ODE for $c_i$ results:
\begin{equation}
    \label{eq:c_i}
    \frac{\d}{\d t}\left( V_i\left( t \right) c_i\left( t \right) \right) =
    \begin{cases}
        \frac{\Gamma_i\left( l_i,t \right) Q_i\left( l_i,t \right)}{A_i\left( l_i,t \right)} - c_i\left( t\right) \cdot \frac{p_{c,i}-p_v}{R_{2,i}}, &\text{ if } Q_i\left( l_i,t \right) \geq 0, \\
        Q_i\left( l_i,t \right) \cdot c_i\left(t\right) - c_i\left( t\right) \cdot \frac{p_{c,i}-p_v}{R_{2,i}}, &\text{ if } Q_i\left( l_i,t \right) < 0.
    \end{cases}
\end{equation}
Solving \eqref{eq:V_i} and \eqref{eq:c_i} for each time point, we have for $\Gamma_i\left( l_i,t \right)$:
\begin{equation}
    \label{eq:gamma_i}
    \Gamma_i\left( l_i,t \right) =
    \begin{cases}
        W_{3,i}\left( l_i,t \right) \cdot A_i\left( l_i,t \right), &\text{ if } Q_i\left( l_i,t \right) \geq 0, \\
        c_i\left( t\right) \cdot A_i\left( l_i,t \right), &\text{ if } Q_i\left( l_i,t \right) < 0.
    \end{cases}
\end{equation}

\section{Additional numerical results} \label{Appendix:Numerical}

Figure~\ref{fig:results3DBreastFlow} depicts the capillary and tissue pressures in the 3D domain. 
The pressure values of both are in the same range for the given parameter values.
This results in slightly larger pressure values near the areola and smaller pressure values towards the human body.
The resulting pressure gradients promote flows from the middle to the upper and lower parts of the breast.

\begin{figure}[htbp]\centering
	\includegraphics[width=0.47\textwidth]{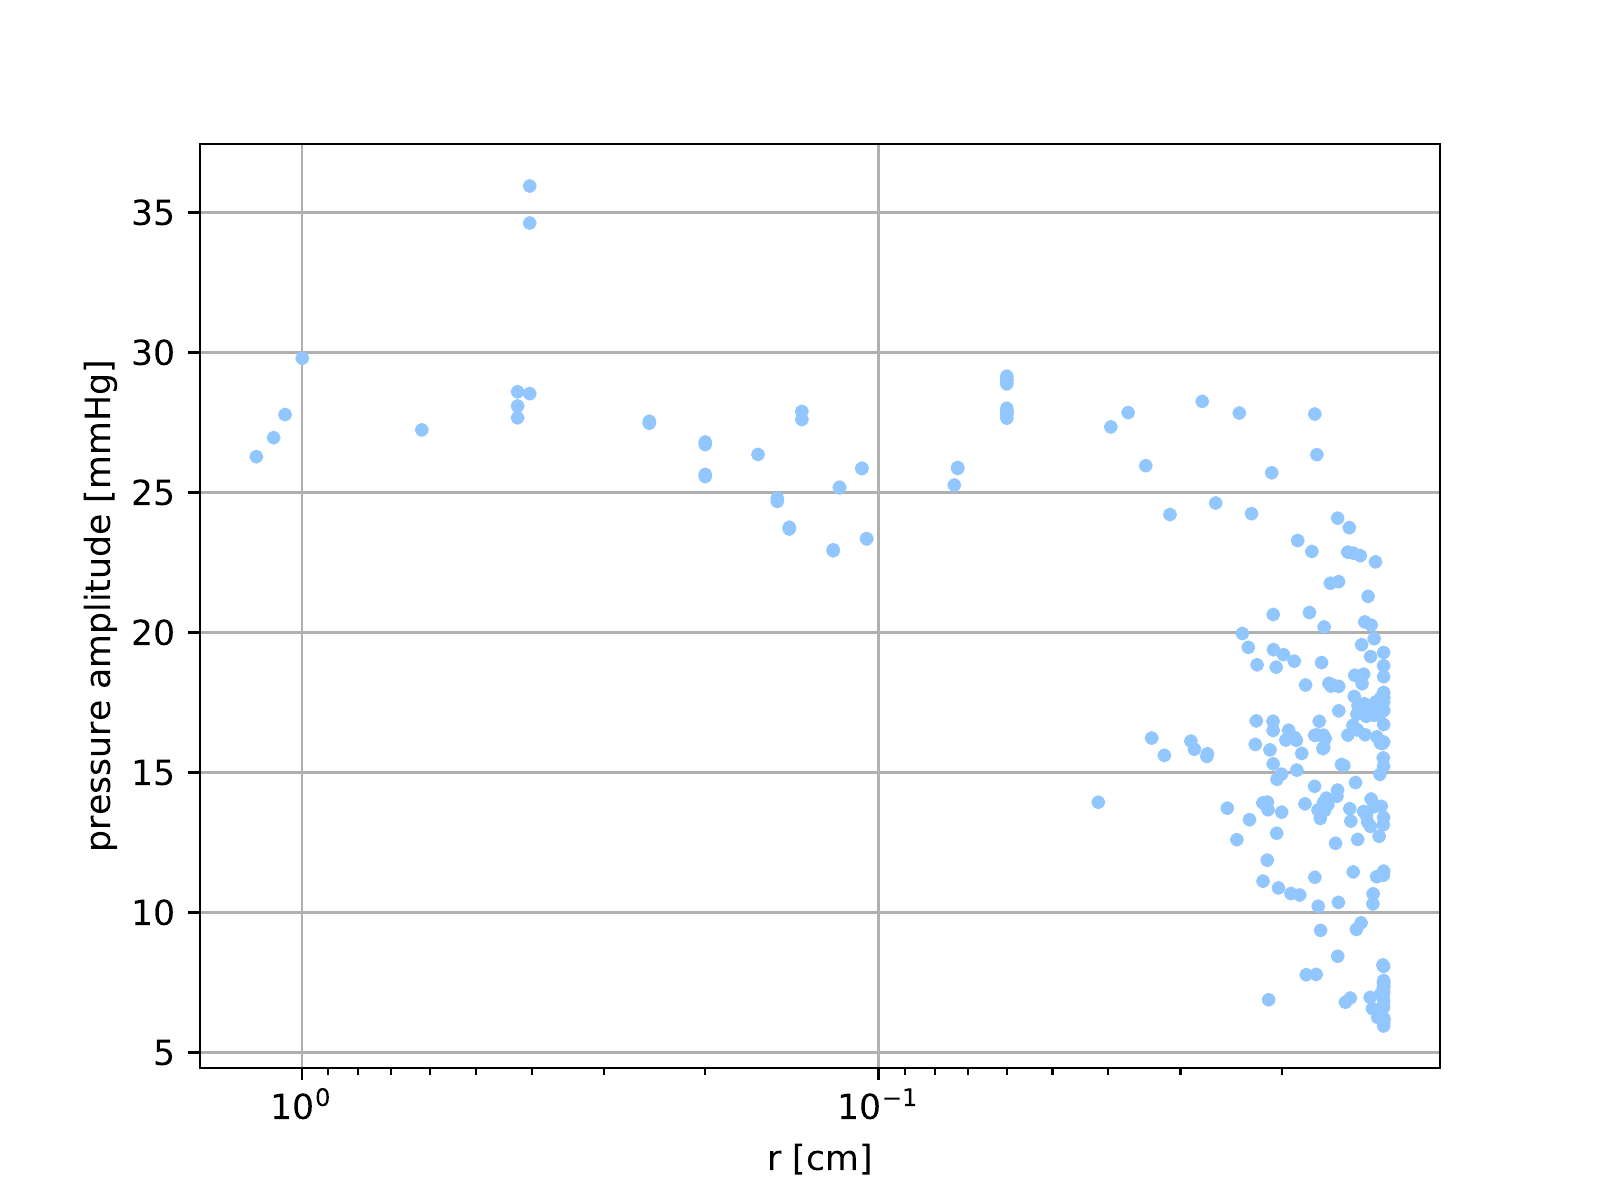}%
	\includegraphics[width=0.48\textwidth]{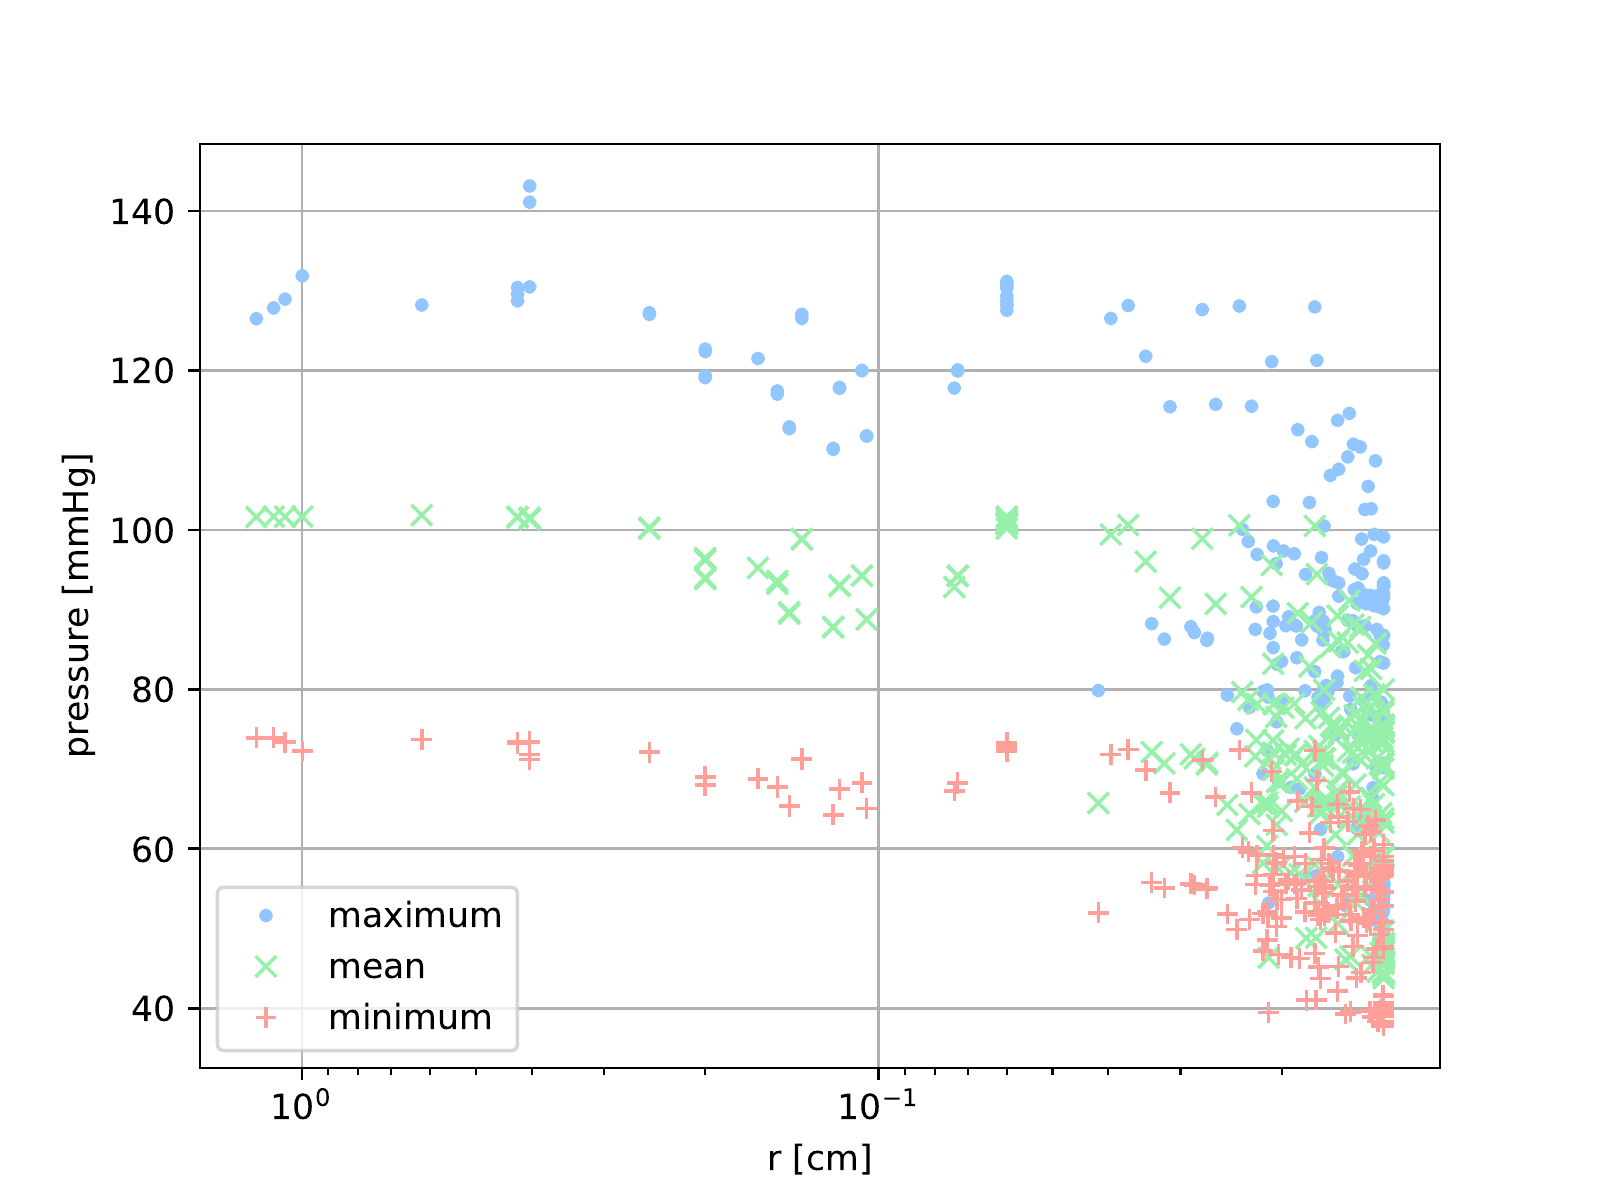}
	\caption{
		\label{fig:results1DAmpMaxMeanMin}
		Plot of the vessel radii at 0 pressure of the nonlinear and linearized flow models against the pressures which were averaged from heart beat 14 to heart beat 20.
		The left figure shows the pressure amplitude in this time interval, while the right shows the maximum, mean and minimum pressures for all radii.}
\end{figure}

\begin{figure}[htbp] \centering
	\includegraphics[width=0.47\textwidth]{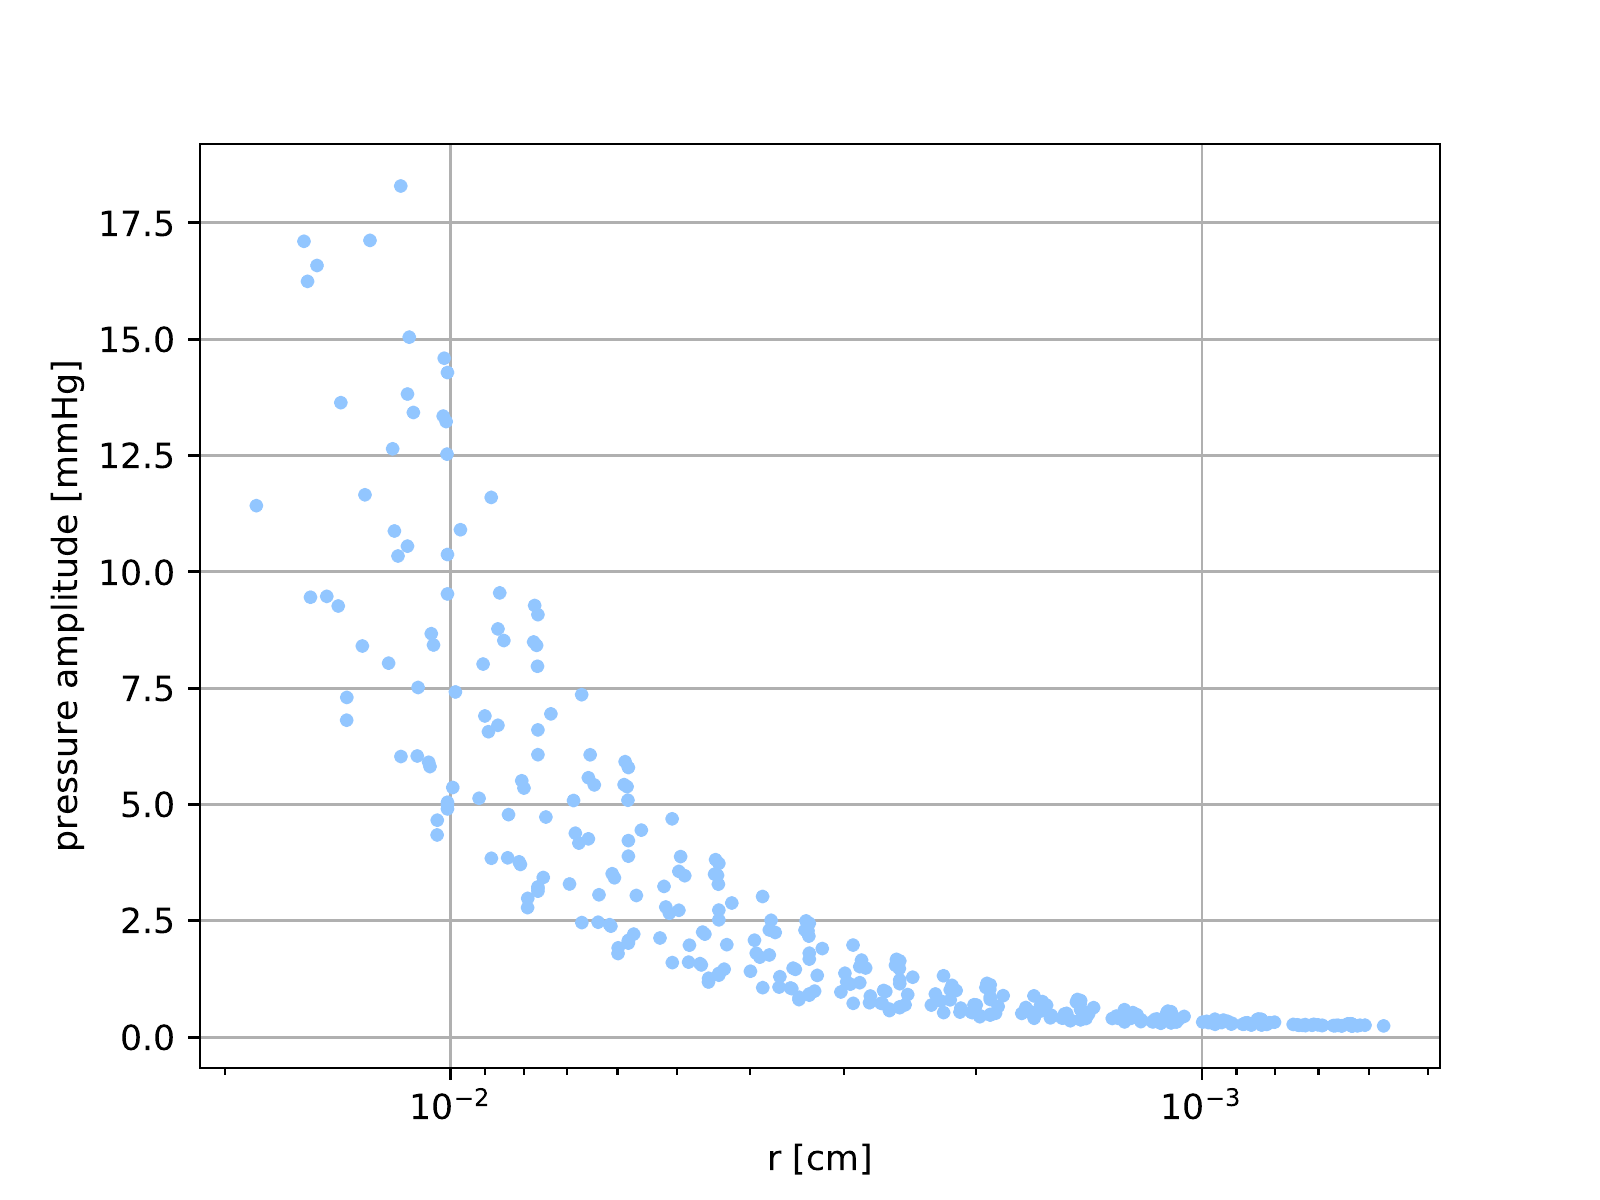}%
	\includegraphics[width=0.47\textwidth]{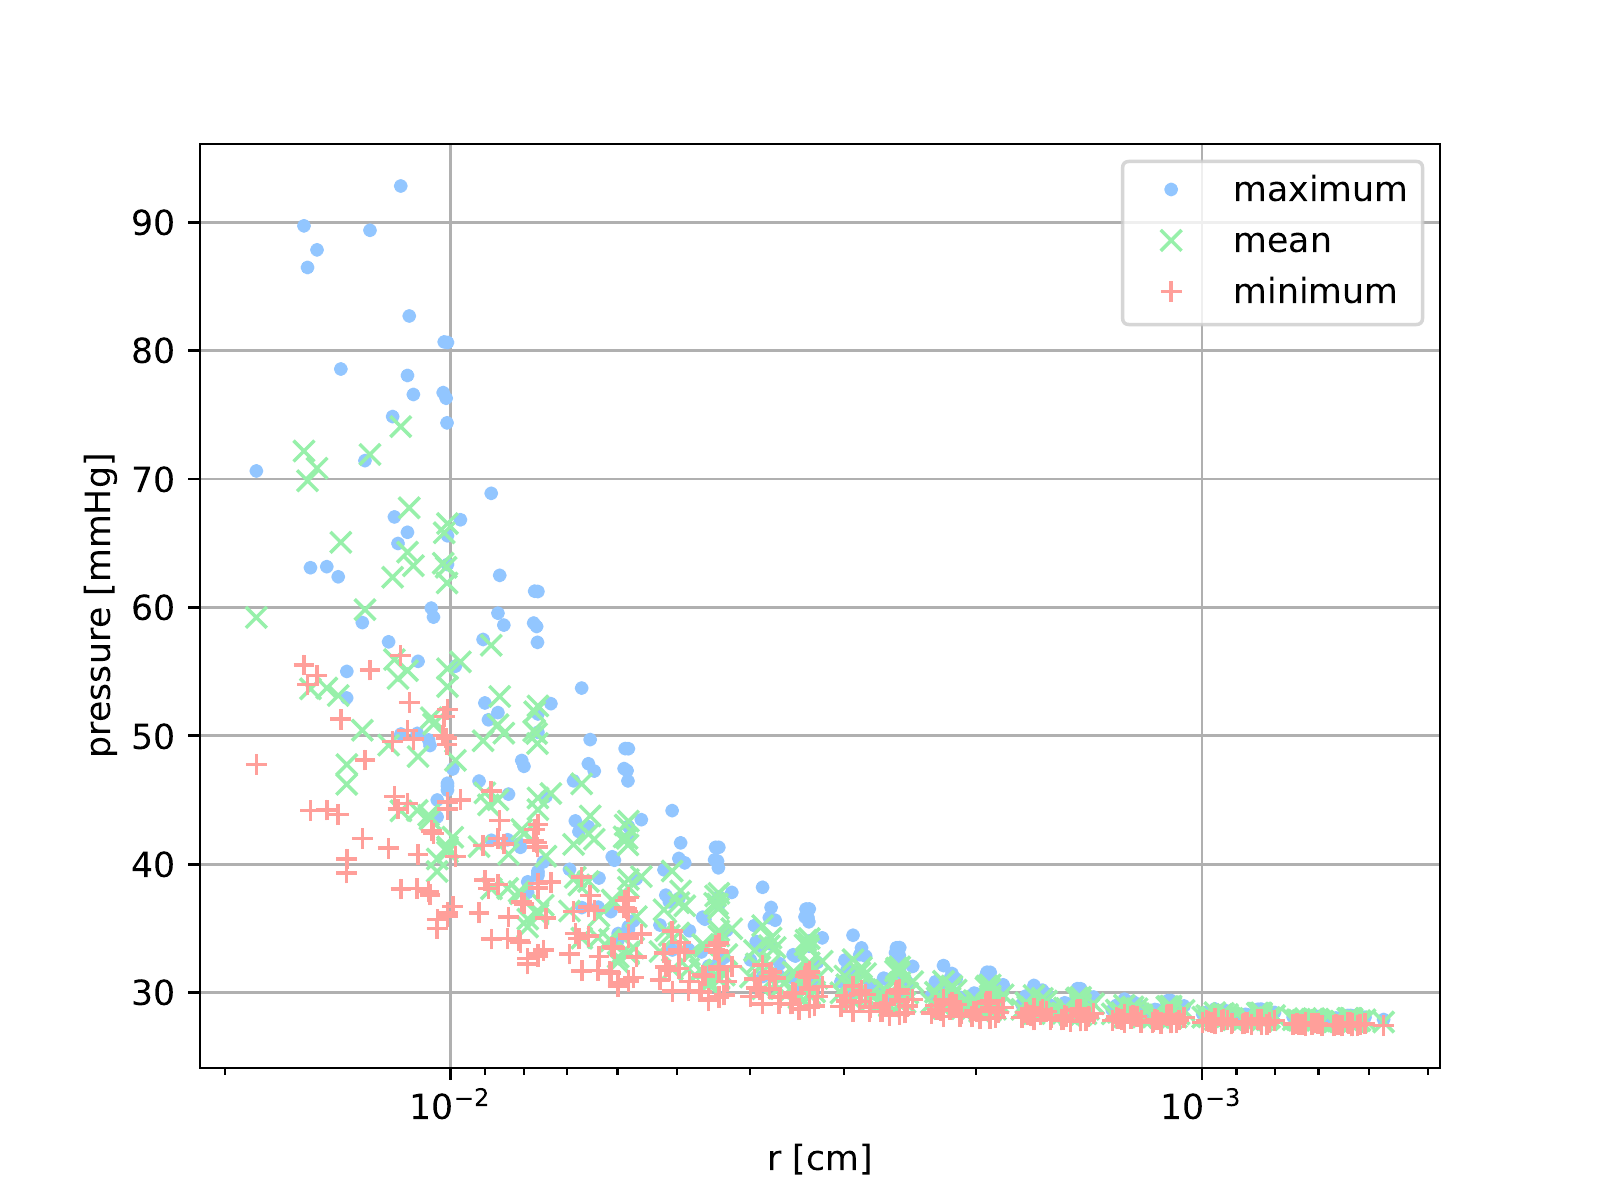}
	\caption{
		\label{fig:results0DAmpMaxMeanMin}
		Plot of the radii of the lumped 0D models against the 0D pressures which were averaged from heart beat 14 to heart beat 20.
		The left figure shows the pressure amplitude in this time interval,
		while the right shows the maximum, mean and minimum pressures for all radii.}
\end{figure}

\begin{figure}[htbp]\centering
	\includegraphics[width=0.5\textwidth]{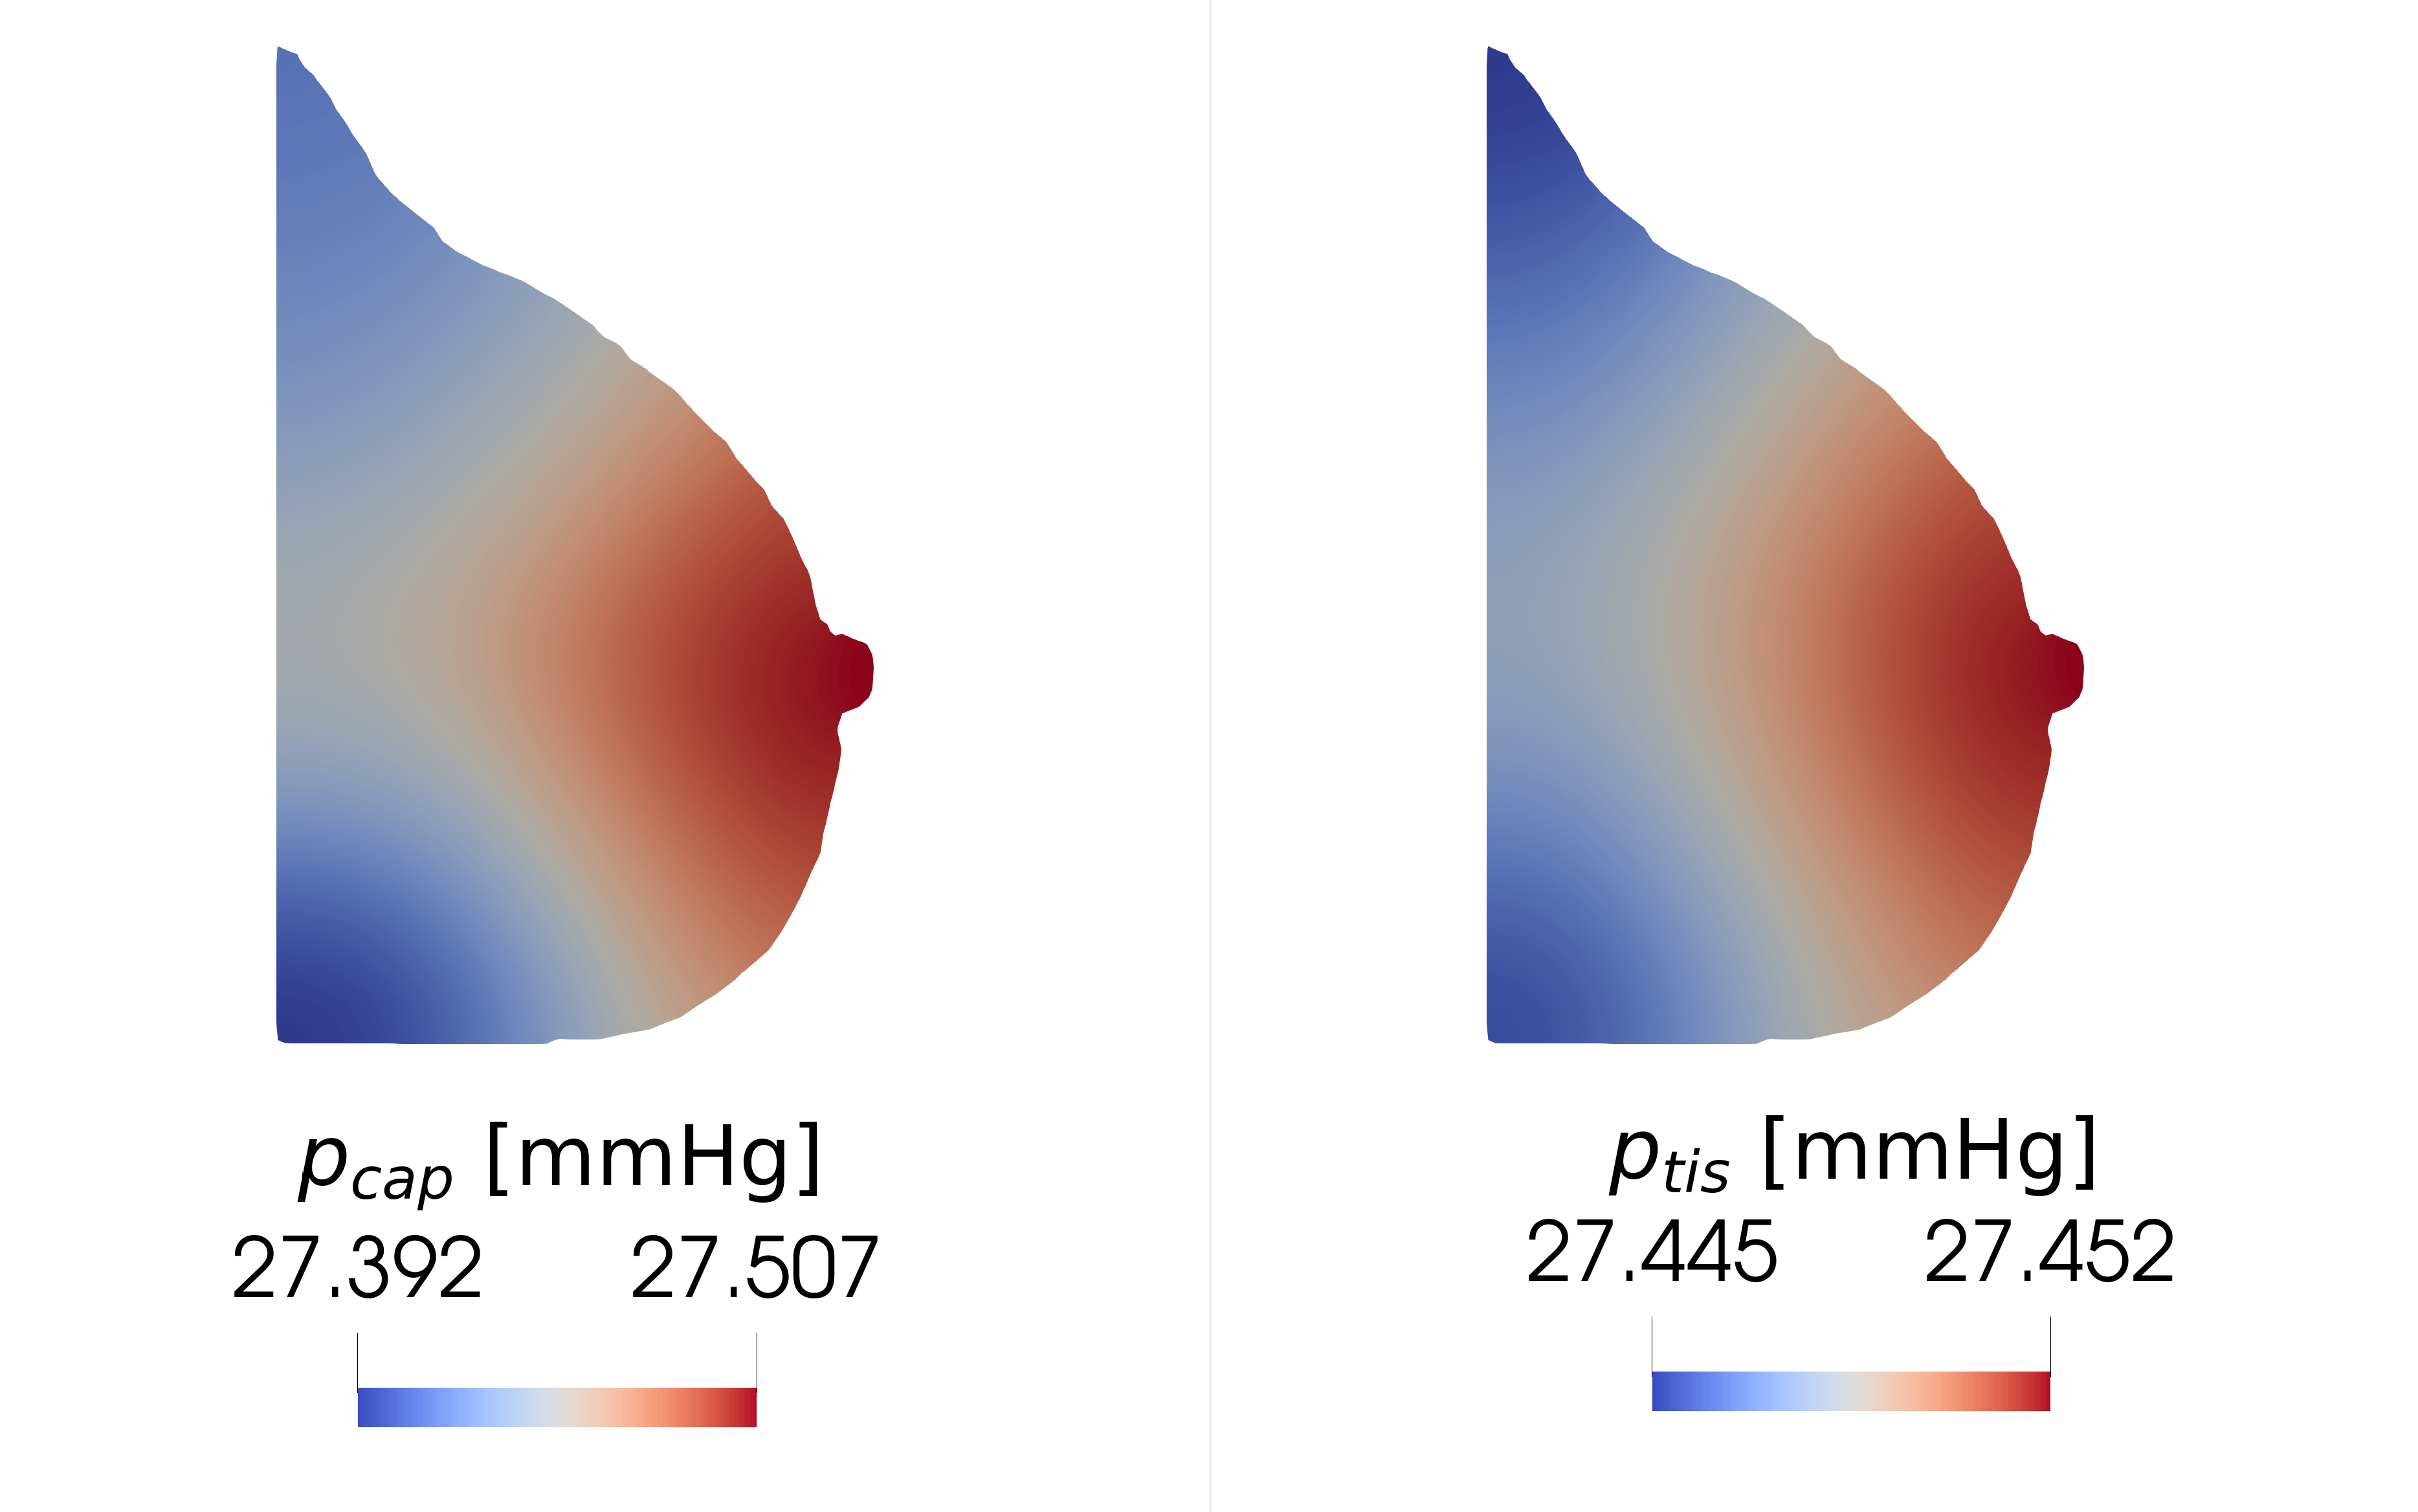}
	\caption{ \label{fig:results3DBreastFlow} Pressure distribution at a fixed time inside the capillary and tissue domains.}
\end{figure}
